# Supplementary material for: DROID: Dose-ranging Approach to Optimizing Dose in Oncology Drug Development
Source: arXiv:2209.01655 source file (2022-09-04)
Supplement: Supplementary file 1 [file DROID-v11-Supp.pdf]

## Supplementary Materials

### 1. Prior specification

For the parameter  $\alpha$  in the logistic model for toxicity, we take  $f(\alpha) = \exp(1)$  as suggested by O'Quigley and Chevret (1991) and Chevret (1993). The prior specification of the parameters in the Emax model for PD is facilitated by their interpretation. For each parameter, we elicit a prior estimate, denoted as  $\hat{\theta}$ , and a range of possible values, denoted as  $(\hat{\theta} - \zeta, \hat{\theta}, +\zeta)$ , from clinicians and assign it a Gamma prior with mean  $\hat{\theta}$  and standard deviation  $\zeta/2$  so that two standard deviations from the mean cover the elicited range. If only the prior estimate is available, we could employ vague priors by assigning each parameter a Gamma prior distribution with mean  $\hat{\theta}$  and a relatively large standard deviation, (e.g.,  $3\hat{\theta}$ ).  $\sigma^2$  is assigned the vague inverse gamma prior  $IG(0.1, 0.1)$ .

### 2. Estimation of ORR $\pi(d_j)$

Suppose that at dose level  $j$ ,  $x_j$  out of  $n_j$  patients have objective response. We adopt the standard Beta-Binomial model by assuming  $x_j \sim \text{Binom}(n_j, \pi(d_j))$  and  $\pi(d_j) \sim \text{Beta}(a, b)$ .  $a$  and  $b$  are hyperparameters which are set at small values, such as  $a=0.1$  and  $b=0.2$ , so that the data will dominate the prior. The raw posterior distribution of  $\pi(d_j)$  is  $\text{Beta}(a + x_j, b + n_j - x_j)$ . To satisfy the ordering constraint that the dose-efficacy curve is non-decreasing, i.e.,  $\pi(d_j) \leq \pi(d_{j+1})$  for any dose level  $j$ , the order-constrained posterior distribution of  $\pi(d_j)$  is obtained through performing isotonic regression to each posterior sample of  $\pi(d_j)$  across all tried dose levels. Dose level  $j$  has acceptable efficacy if  $\Pr(\pi(d_j) > \phi_E | D) > C_E$  where  $C_E$  is a

probability cutoff to be tuned through simulation. Efficacy acceptability can also be defined using point estimate, i.e., dose level  $j$  has acceptable efficacy if  $\hat{\pi}(d_j) > \phi_E$ .

### 3. Using Bayesian model averaging (BMA) to consider multiple dose-response models

Another advantage of DRI is that it is straightforward for it to account for the uncertainty of the dose-response model using Bayesian model averaging (BMA) to improve the robustness of the inference. Following the similar spirit of MCP-Mod, we could consider multiple candidate dose-response models (e.g., Emax model, linear model, exponential model), denoted as  $M_1, \dots, M_K$ . The BMA estimate of DRI is given by  $DRI = \sum_{k=1}^K \Pr(M_k|data)DRI_k$ , where  $DRI_k$  is the DRI calculated under  $M_k$ , and  $\Pr(M_k|data)$  is the posterior probability of  $M_k$  being true given the data. The BMA of the dose-response curve is given by  $\hat{\mu}(d) = \sum_{k=1}^K \Pr(M_k|D)\hat{\mu}(d|M_k)$ , where  $\hat{\mu}(d|M_k)$  is the estimate of PD given  $M_k$ . In contrast, it is challenging to make similar inferences under the frequentist approach. Although technically the BMA approach may also be used in stage I TDR finding to account for modelling uncertainty, it may not be useful due to limited data observed in stage I. In small sample size dose finding studies, parsimonious model often outperforms complicated model (Cheung, 2011; Iasonos, et al., 2016).

### 4. Selection percentage and the average number of patients treated at each dose under DROID-BOIN based on ORR that selects $d_{opt}$ as the dose where $\pi(d_j)$ plateaus under two cutoff values for $C_1$ .

| Dose level   | 1                            | 2            | 3     | 4     | 5     | 1                           | 2            | 3     | 4     | 5     |
|--------------|------------------------------|--------------|-------|-------|-------|-----------------------------|--------------|-------|-------|-------|
|              | <u><math>C_1=0.85</math></u> |              |       |       |       | <u><math>C_1=0.7</math></u> |              |       |       |       |
|              | scenario 1                   |              |       |       |       |                             |              |       |       |       |
| Sel %        | 0.002                        | <b>0.359</b> | 0.544 | 0.048 | 0.000 | 0.022                       | <b>0.600</b> | 0.314 | 0.017 | 0.000 |
| no. patients | 19.9                         | <b>19.8</b>  | 18.5  | 14.8  | 4.2   | 19.9                        | <b>19.8</b>  | 18.5  | 14.8  | 4.2   |

|              |              |              |              |              |              |              |              |              |              |              |
|--------------|--------------|--------------|--------------|--------------|--------------|--------------|--------------|--------------|--------------|--------------|
|              |              |              |              |              | scenario 2   |              |              |              |              |              |
| Sel %        | 0.000        | 0.158        | <b>0.576</b> | 0.238        | 0.002        | 0.004        | 0.368        | <b>0.503</b> | 0.099        | 0.000        |
| no. patients | 19.4         | 19.8         | <b>19.4</b>  | 18.3         | 10.4         | 19.4         | 19.8         | <b>19.4</b>  | 18.3         | 10.4         |
|              |              |              |              |              | scenario 3   |              |              |              |              |              |
| Sel %        | 0.000        | 0.104        | <b>0.630</b> | 0.257        | 0.003        | 0.003        | 0.266        | <b>0.619</b> | 0.105        | 0.001        |
| no. patients | 19.3         | 20.0         | <b>19.5</b>  | 18.2         | 10.9         | 19.3         | 20.0         | <b>19.5</b>  | 18.2         | 10.9         |
|              |              |              |              |              | scenario 4   |              |              |              |              |              |
| Sel %        | 0.000        | 0.000        | 0.117        | <b>0.639</b> | 0.241        | 0.000        | 0.014        | 0.408        | <b>0.496</b> | 0.079        |
| no. patients | 13.7         | 18.7         | 19.9         | <b>19.9</b>  | 18.8         | 13.7         | 18.7         | 19.9         | <b>19.9</b>  | 18.8         |
|              |              |              |              |              | scenario 5   |              |              |              |              |              |
| Sel %        | 0.000        | 0.021        | 0.254        | <b>0.656</b> | 0.064        | 0.000        | 0.032        | 0.501        | <b>0.450</b> | 0.012        |
| no. patients | 14.1         | 19.4         | 19.7         | <b>18.6</b>  | 11.8         | 14.1         | 19.4         | 19.7         | <b>18.6</b>  | 11.8         |
|              |              |              |              |              | scenario 6   |              |              |              |              |              |
| Sel %        | 0.013        | <b>0.837</b> | 0.094        | 0.000        | 0.000        | 0.077        | <b>0.818</b> | 0.049        | 0.000        | 0.000        |
| no. patients | 20.1         | <b>19.9</b>  | 12.3         | 1.5          | 0.0          | 20.1         | <b>19.9</b>  | 12.3         | 1.5          | 0.0          |
|              |              |              |              |              | scenario 7   |              |              |              |              |              |
| Sel %        | 0.000        | 0.000        | 0.020        | 0.403        | <b>0.571</b> | 0.000        | 0.002        | 0.092        | 0.561        | <b>0.339</b> |
| no. patients | 8.3          | 15.6         | 19.8         | 19.9         | <b>18.6</b>  | 8.3          | 15.6         | 19.8         | 19.9         | <b>18.6</b>  |
|              |              |              |              |              | scenario 8   |              |              |              |              |              |
| Sel %        | <b>0.577</b> | 0.290        | 0.000        | 0.000        | 0.000        | <b>0.592</b> | 0.275        | 0.000        | 0.000        | 0.000        |
| no. patients | <b>22.9</b>  | 15.3         | 2.5          | 0.3          | 0.0          | <b>22.9</b>  | 15.3         | 2.5          | 0.3          | 0.0          |
|              |              |              |              |              | scenario 9   |              |              |              |              |              |
| Sel %        | 0.000        | 0.387        | 0.395        | 0.027        | 0.000        | 0.025        | 0.621        | 0.155        | 0.008        | 0.000        |
| no. patients | 19.9         | 19.9         | 19.8         | 18.5         | 5.5          | 19.9         | 19.9         | 19.8         | 18.5         | 5.5          |
